# Supplementary material for: FocusMAE: Gallbladder Cancer Detection from Ultrasound Videos with Focused Masked Autoencoders
Source: arXiv:2403.08848 source file (2024-03-29)
Supplement: Supplementary file 1 [file table-supp-img-baselines.tex]

\begin{table*}[t]
\centering
%\scriptsize
%\setlength{\tabcolsep}{4pt}
\resizebox{ \linewidth}{!}{%
\begin{tabular}{p{0.12\linewidth}p{0.38\linewidth}p{0.08\linewidth}p{0.2\linewidth}p{0.05\linewidth}p{0.06\linewidth}}
\toprule[1.5pt]
\textbf{Model} & \textbf{Description} & \textbf{Input Size} & \textbf{Optimizer} & \textbf{Batch size} & \textbf{Epochs/ Steps}
\\ \midrule[0.75pt]
YOLOv4 \cite{yolov4} & CSPDarknet53 backbone, PANet neck, anchor-based YOLO head. Total 162-layers. Backbone was frozen for first 800 step. Entire network was trainable thereafter. Single stage, anchor-based  & $608\times608\times3$ & SGD LR = 0.0001 momentum = 0.95 weight decay = 0.0005 & 64 & 3000 steps \\ \midrule
Faster-RCNN \cite{fasterrcnn} & Resnet50 Feature Pyramid backbone. Backbone was frozen for training. Two-stage, anchor-based. & $800 \times 1333 \times 3$ & SGD LR = 0.005 momentum = 0.9 weight decay = 0.0005 & 16 & 60 epochs \\ \midrule
Reppoints \cite{reppoints} & Resnet101 backbone, Group Normalization neck, and a reppoints head. Backbone was frozen for first 30 epochs, and entire network was trainable thereafter. Two-stage, anchor-free & $800 \times 1333 \times 3$ & SGD LR = 0.001 momentum = 0.9 weight decay = 0.0001 & 4 & 50 epochs \\ \midrule
Centripetal-Net \cite{centripetalnet} & Improvement over CornerNet model. Uses centripetal shift to match corners. HourglassNet-104 backbone. Enitre network was trainable. Anchor-free & $511 \times 511 \times 3$ & Adam LR = 0.0005 & 4 & 50 epochs \\ \midrule
ResNet \cite{resnet} & Resnet-50 used. All layers were trainable. Output dimension of last fully connected layer is three - corresponding to normal, benign, and malignant GB. LR decays by 10\% after every 5 epochs through a step LR scheduler. & $224\times224\times3$ & SGD LR = 0.005 momentum = 0.9 weight decay = 0.0005 & 16 & 100 epochs \\ \midrule
Inception \cite{inception} & Inception-V3 used. All layers were trainable. LR decays by 10\% after every 5 epochs through a step LR scheduler. & $299\times299\times3$ & SGD LR = 0.005 momentum = 0.9 weight decay = 0.0005 & 16 & 100 epochs \\ \midrule
EfficientDet \cite{efficientdet} & EfficientNet-B4 used as backbone and BiFPN as feature network. All layers were trainable. Three output classes corresponding to normal, benign, and malignant GB. & $1024\times1024\times3$ & Adam LR = 0.001 & 2 & 50 epochs \\ %\midrule
\bottomrule
\end{tabular}
}
\caption{Implementation details for the image-based baseline networks.}
\label{tab:configs}
\end{table*}
