# Supplementary material for: FocusMAE: Gallbladder Cancer Detection from Ultrasound Videos with Focused Masked Autoencoders
Source: arXiv:2403.08848 source file (2024-03-29)
Supplement: Supplementary file 2 [file table-supp-hyper.tex]

\begin{table*}[ht]
	\centering
    \small
	%\resizebox{ \linewidth}{!}{%
	\begin{tabular}{cccccccc}
		\toprule
		\multirow{3}{*}{\textbf{Masking Ratio}} & \multirow{3}{*}{\textbf{Decoder Depth}} & \multicolumn{6}{c}{\textbf{Loss}} \\
        & & \multicolumn{3}{c}{\textbf{MSE}} & \multicolumn{3}{c}{\textbf{L1}} \\
        & & Acc. & Spec. & Sens. & Acc. & Spec. & Sens. \\
        %& {\textbf{Time/Frame (ms)}}\\
		\midrule
        \multirow{4}{*}{0.6}
		& 4  & 0.538$\pm$0.443 & 0.808$\pm $0.123& 0.940$\pm$0.120 & 0.943$\pm$0.065 
         & 0.940$\pm$0.120 & 0.938$\pm$0.076 \\
  
        & 6 & 0.945$\pm$0.071 & 0.940$\pm$0.120 & 1.000$\pm$0.000 & 0.943$\pm$0.065& 0.940$\pm$0.120& 0.938$\pm$0.076  \\
        
        & 8 & 0.942$\pm$0.066 & 0.940$\pm$0.120 & 0.938$\pm$0.076& 0.943$\pm$0.065 & 0.940$\pm$0.120 & 0.938$\pm$0.076  \\
        
        & 10 & 0.749$\pm$0.144 & 0.940$\pm$0.120 & 0.600$\pm$0.490  & 0.943$\pm$0.065 & 0.940$\pm$0.120 & 0.938$\pm$0.076  \\
        \midrule 
		\multirow{4}{*}{0.8}
		& 4 & 0.940$\pm$0.066  & 0.940$\pm$0.120& 0.938$\pm$0.076 & 0.86$\pm$0.124 & 0.699$\pm$0.371 & 0.940$\pm$0.120 \\
        & 6 & 0.942$\pm$0.065  & 0.940$\pm$0.120 & 0.938$\pm$0.076 & 0.943$\pm$0.065 & 1.000$\pm$0.000 & 0.938$\pm$0.076 \\
        & 8 & 0.942$\pm$0.066 & 0.940$\pm$0.120 & 0.938$\pm$0.076 & 0.978$\pm$0.027 & 1.000$\pm$0.000 & 0.938$\pm$0.076\\
        & 10 & 0.952$\pm$0.070 & 0.940$\pm$0.120 & 0.967$\pm$0.067 & 0.943$\pm$0.065 & 0.940$\pm$0.120 & 0.938$\pm$0.076 \\
        \midrule 
        \multirow{4}{*}{0.95}
		& 4 & 0.810$\pm$0.124 &0.940$\pm$0.120& 0.538$\pm$0.443 & 0.943$\pm$0.065 &0.940$\pm$0.120 & 0.938$\pm$0.076 \\
        & 6 & 0.943$\pm$0.065 & 0.940$\pm$0.120 & 0.938$\pm$0.076& 0.943$\pm$0.065 & 0.940$\pm$0.120 & 0.938$\pm$0.076 \\
        & 8 & 0.811$\pm$0.122&0.940$\pm$0.120 & 0.538$\pm$0.443 & 0.943$\pm$0.065 & 0.940$\pm$0.120 & 0.938$\pm$0.076 \\
        & 10 & 0.964$\pm$0.072 & 0.940$\pm$0.120 & 1.000$\pm$0.000 & 0.943$\pm$0.065& 0.094$\pm$0.120 & 0.938$\pm$0.076 \\
		%
  %       \midrule 
  %       %
  %       \multirow{4}{*}{1}
		% & 4 & 0.966$\pm$0.028 & 1.000$\pm$0.000 & 0.909$\pm$0.074 & 0.965$\pm$0.071 & 0.940$\pm$0.120 & 1.000$\pm$0.000 \\
  %       & 6 & 0.943$\pm$0.065 & 0.940$\pm$0.120& 0.938$\pm$0.076 &0.943$\pm$0.065 &1.000$\pm$0.000 &0.938$\pm$0.076  \\
  %       & 8 & 0.943$\pm$0.065 & 0.940$\pm$0.120 & 0.938$\pm$0.076 & 0.943$\pm$0.065 &1.000$\pm$0.000 &0.938$\pm$0.076  \\
  %       & 10 & 0.966$\pm$0.028 & 1.000$\pm$0.000 & 0.91$\pm$0.074 & 0.943$\pm$0.065 &1.000$\pm$0.000 &0.938$\pm$0.076 \\
		\bottomrule
	\end{tabular}
	%}
	\caption{Hyperparameter tuning. We vary the Masking ratio, Decoder depth, and the loss function for a grid search. We report the 5-fold cross-validation (Mean$\pm$SD) accuracy, specificity, and sensitivity for \myarch in detecting GBC from the US. 
    }
	\label{tab:hyperparam_supp}
\end{table*}
